# Supplementary material for: Image Generation Via Minimizing Fr\'echet Distance in Discriminator Feature Space
Source: arXiv:2003.11774 source file (2020-03-30)
Supplement: Supplementary file 1 [file appendix.tex]

\section*{Appendix}

\subsection{Supported mathematical results}

We collect below, several mathematical results that are useful for this paper.

\begin{theorem}
A positive semi-definite square matrix $A$ has a unique semi-definite symmetric square root, called the \textit{principal square root}. 
\label{theorem:unique_square_root}
\end{theorem}

\begin{proof}
In Section~\ref{subsubsec:computing_squareroot}, we show the existence of the square root matrix $B$ of the Positive Semi-Definite matrix $A$. Now we prove that $B$ is unique.

Suppose that there exists a real positive semi-definite, symmetric matrix $C$ that also a square root matrix of $A$. $C$ can be diagonalized with a orthogonal matrix $P$ such that $P^T C P = \Sigma'$, where $\Sigma'$ is a diagonal matrix whose diagonal entries $\alpha_1,...,\alpha_d$ are the eigenvalues of $C$.

We can also derive $P^T A P = P^T C^2 P = (P^T C P)^2 = T^2$. Hence, $P$ also diagonalizes $A$. It follows that $\alpha_1^2,...,\alpha_d^2$ equal $\lambda_1,...,\lambda_d$ (the eigenvalues of $A$), up to a permutation. Thus, we can arrange the columns of $P$ so that $P^T C P = \Sigma'$.

Furthermore, since $B^2 = C^2$, we have:

\begin{align}
             & (S^T \Sigma' S) = (P^T \Sigma' P)^2 \\
    \Leftrightarrow & S^T \Sigma'^2 S = P^T \Sigma'^2 P \\
    \Leftrightarrow & S^T \Sigma S = P^T \Sigma P \\
    \Leftrightarrow & (P^T S) \Sigma = \Sigma (P^T S) \\
    \Leftrightarrow & Q \Sigma = \Sigma Q \\
\end{align}

where $Q = P^T S$. 

Without loss of generality, we assume that $\Sigma$ is a block diagonal matrix as follows:

\begin{equation*}
\Sigma = 
\begin{pmatrix}
\lambda_1 I_1 & 0 & \cdots & 0 \\
0 & \lambda_2 I_2 & \cdots & \vdots \\
\vdots  & \vdots  & \ddots & \vdots  \\
0 & \cdots & 0 & \lambda_k I_k
\end{pmatrix}
\end{equation*}

where $\lambda_k$'s are unique eigenvalues of $A$ and $I_k$ is some Identity matrix whose size equals the algebraic multiplicity of $\lambda_k$. Similarly, we can also express $Q$ as a block matrix with the same partition as $\Sigma$:

\begin{equation*}
Q = 
\begin{pmatrix}
Q_{11} & Q_{12} & \cdots & Q_{1k} \\
Q_{21} & Q_{22} & \cdots & \vdots \\
\vdots  & \vdots  & \ddots & \vdots  \\
Q_{k1} & \cdots & 0 & Q_{kk}
\end{pmatrix}
\end{equation*}

Because $Q \Sigma = \Sigma Q$, we have $\lambda_i Q_{ii} = Q_{ii} \lambda_i$ and $Q_{ij} = 0$ for $i \ne j$.

Since $\Sigma'$ can also be expressed as a block diagonal matrix with the same partition, we can show that $Q \Sigma' = \Sigma' Q$. Hence, $\Sigma' = Q^T \Sigma' Q$ since $Q$ is also an orthogonal matrix. 

Finally, we can show that:

\begin{align}
    B &= S \Sigma' S^T = S (Q^T \Sigma' Q) S \\
      &= S S^T P \Sigma' P^T S S^T \\
      &= P \Sigma' P^T = C
\end{align}

Therefore, any square root matrix $C$ must equal to $B$. This completes the proof of uniqueness.
\end{proof}

\begin{theorem}
The data covariance matrices $\Sigma_d^{D'}$ and  $\Sigma_g^{D'}$ are positive semi-definite symmetric. 
\label{theorem:psd_covariance}
\end{theorem}

\begin{proof}
Let $X \in \mathcal{R}^{N \times d}$ be the data matrix. Without loss of generality, we can assume that the mean vector $\mu = 0$ (otherwise we can subtract $\mu$ from $X$). Then, the covariance matrix is $\Sigma = E[XX^T]$, which is also a symmetric matrix.

For any vector $u \in \mathcal{R}^d$, we have:
\begin{equation}
    u^T \Sigma u = u^T E[X X^T] u = E[u^T X X^T u] = E[(X^T u)^2] \ge 0
\end{equation}

Hence, the data covariance matrix $\Sigma$ is positive semi-definite matrix.

\end{proof}

% \begin{corollary}
% There exists a unique square root for  $\Sigma_d^{D'}\Sigma_g^{D'}$.
% \label{cor:unique}
% \end{corollary}

% \begin{proof}
% From Theorem~\ref{theorem:psd_covariance}, $\Sigma_d^{D'}$ and $\Sigma_g^{D'}$ are symmetric, positive semi-definite matrices. Hence, $\Sigma_d^{D'}\Sigma_g^{D'}$ is also positive semi-definite. From Theorem~\ref{theorem:unique_square_root}, $\Sigma_d^{D'}\Sigma_g^{D'}$ always has a unique square root.
% \end{proof}

\subsection{Additional synthetic experiments}

In this section, we present additional results for generating synthetic data. We consider two synthetic datasets, which are widely used in the GAN literature. The first dataset is 25-Gaussians, which consists of 25 gaussian modes in a two-dimensional grid layout. The second dataset is Swissroll, in which the data follows a two-dimensional spiral-layered shape, similar to the layers in a Swissroll. Figures~\ref{fig:synthetic_gaussian_25} and~\ref{fig:synthetic_swissroll} show the results of generating the 25-Gaussians and Swissroll data, respectively. Also, we show more baselines in this experiment, including the original Non-saturating GAN, and Least-Square GAN (LS-GAN). 

We observer similar results to the 8-Gaussian experiment. 

\begin{table*}[!ht]

\centering
\begin{tabularx}{\textwidth}{c|c}
% \hline
% \rotatebox{90}{\parbox{1.5cm}{\textbf{SWG+D}}} &
\includegraphics[width=2.4in]{figures/gaussian_25/z_dim-10-unrolled_steps-5-prior_std-0.00-Non-Saturating.png}
&
\includegraphics[width=2.4in]{figures/gaussian_25/z_dim-10-unrolled_steps-5-prior_std-0.00-LS-GAN.png}
\\
\includegraphics[width=2.4in]{figures/gaussian_25/z_dim-10-unrolled_steps-5-prior_std-0.00-WGAN.png}
&
\includegraphics[width=2.4in]{figures/gaussian_25/z_dim-10-unrolled_steps-5-prior_std-0.00-WGAN-GP.png}
\\
\includegraphics[width=2.4in]{figures/gaussian_25/z_dim-10-unrolled_steps-5-prior_std-0.00-SWG.png}
& \includegraphics[width=2.4in]{figures/gaussian_25/z_dim-10-unrolled_steps-5-prior_std-0.00-SWG-With-D.png}
\\
\includegraphics[width=2.4in]{figures/gaussian_25/z_dim-10-unrolled_steps-5-prior_std-0.00-LP-512.png}
&
\includegraphics[width=2.4in]{figures/gaussian_25/z_dim-10-unrolled_steps-5-prior_std-0.00-LP-With-D-512.png}
\\
\includegraphics[width=2.4in]{figures/gaussian_25/z_dim-10-unrolled_steps-5-prior_std-0.00-M-SWG.png}
&
\includegraphics[width=2.4in]{figures/gaussian_25/z_dim-10-unrolled_steps-5-prior_std-0.00-FGD-With-D.png}
\\
\end{tabularx}
\caption{Dynamic results of 25-Gaussian estimation. The blue $+$ markers are the means of the Gaussians}
\label{fig:synthetic_gaussian_25}
\end{table*}

\begin{table*}[!h]
\centering
\begin{tabularx}{\textwidth}{c|c}
% \hline
% \rotatebox{90}{\parbox{1.5cm}{\textbf{SWG+D}}} &
\includegraphics[width=2.4in]{figures/swissroll/z_dim-10-unrolled_steps-5-prior_std-0.00-Non-Saturating.png}
&
\includegraphics[width=2.4in]{figures/swissroll/z_dim-10-unrolled_steps-5-prior_std-0.00-LS-GAN.png}
\\
\includegraphics[width=2.4in]{figures/swissroll/z_dim-10-unrolled_steps-5-prior_std-0.00-WGAN.png}
&
\includegraphics[width=2.4in]{figures/swissroll/z_dim-10-unrolled_steps-5-prior_std-0.00-WGAN-GP.png}
\\
\includegraphics[width=2.4in]{figures/swissroll/z_dim-10-unrolled_steps-5-prior_std-0.00-SWG.png}
& \includegraphics[width=2.4in]{figures/swissroll/z_dim-10-unrolled_steps-5-prior_std-0.00-SWG-With-D.png}
\\
\includegraphics[width=2.4in]{figures/swissroll/z_dim-10-unrolled_steps-5-prior_std-0.00-LP-512.png}
&
\includegraphics[width=2.4in]{figures/swissroll/z_dim-10-unrolled_steps-5-prior_std-0.00-LP-With-D-512.png}
\\
\includegraphics[width=2.4in]{figures/swissroll/z_dim-10-unrolled_steps-5-prior_std-0.00-M-SWG.png}
&
\includegraphics[width=2.4in]{figures/swissroll/z_dim-10-unrolled_steps-5-prior_std-0.00-FGD-With-D.png}
\\
\end{tabularx}
\caption{Dynamic results of Swissroll estimation. The blue columns (blue) show the Target data for reference.}
\label{fig:synthetic_swissroll}
\end{table*}

\subsection{Training Time}

In this experiment, we present the training time per epoch of the methods. For each method, we collect the training time in seconds per epoch for several epochs on the CIFAR-10 dataset.  Figure~\ref{subfig-1:time_all} shows the training time of OT-GAN and Fr\'{e}chet-GAN, compared to the baselines. While OT-GAN has the worst computational efficiency, Fr\'{e}chet-GAN's computational efficiency is comparable to other GANs. In Figures~\ref{subfig-2:time_lp} and~\ref{subfig-2:time_fgd}, we observe that the training time of Fr\'{e}chet-GAN is not sensitive to the mini-batch as OT-GAN. Specifically, as the mini-batch size increases, the computation complexity of OT also increases while the computation complexity of Fr\'{e}chet-GAN decreases. We also observe that the Fr\'{e}chet-GAN's generalization is not sensitive to the batch-size, as shown in Figure~\ref{subfig-2:fgd_batch_size_fid}. One important conclusion from this experiment: we can train larger batch-sizes in Fr\'{e}chet-GAN. Recently, larger batch-size training is preferred because it leads to to greater parallelism and shorter training time of the models~\cite{smith2017don}.

\begin{figure*}[!h]
 \setcounter{figure}{9}       
 \centering
 
 \subfloat[All Methods: Training Time \label{subfig-1:time_all}]{%
  \includegraphics[width=0.8 \textwidth]{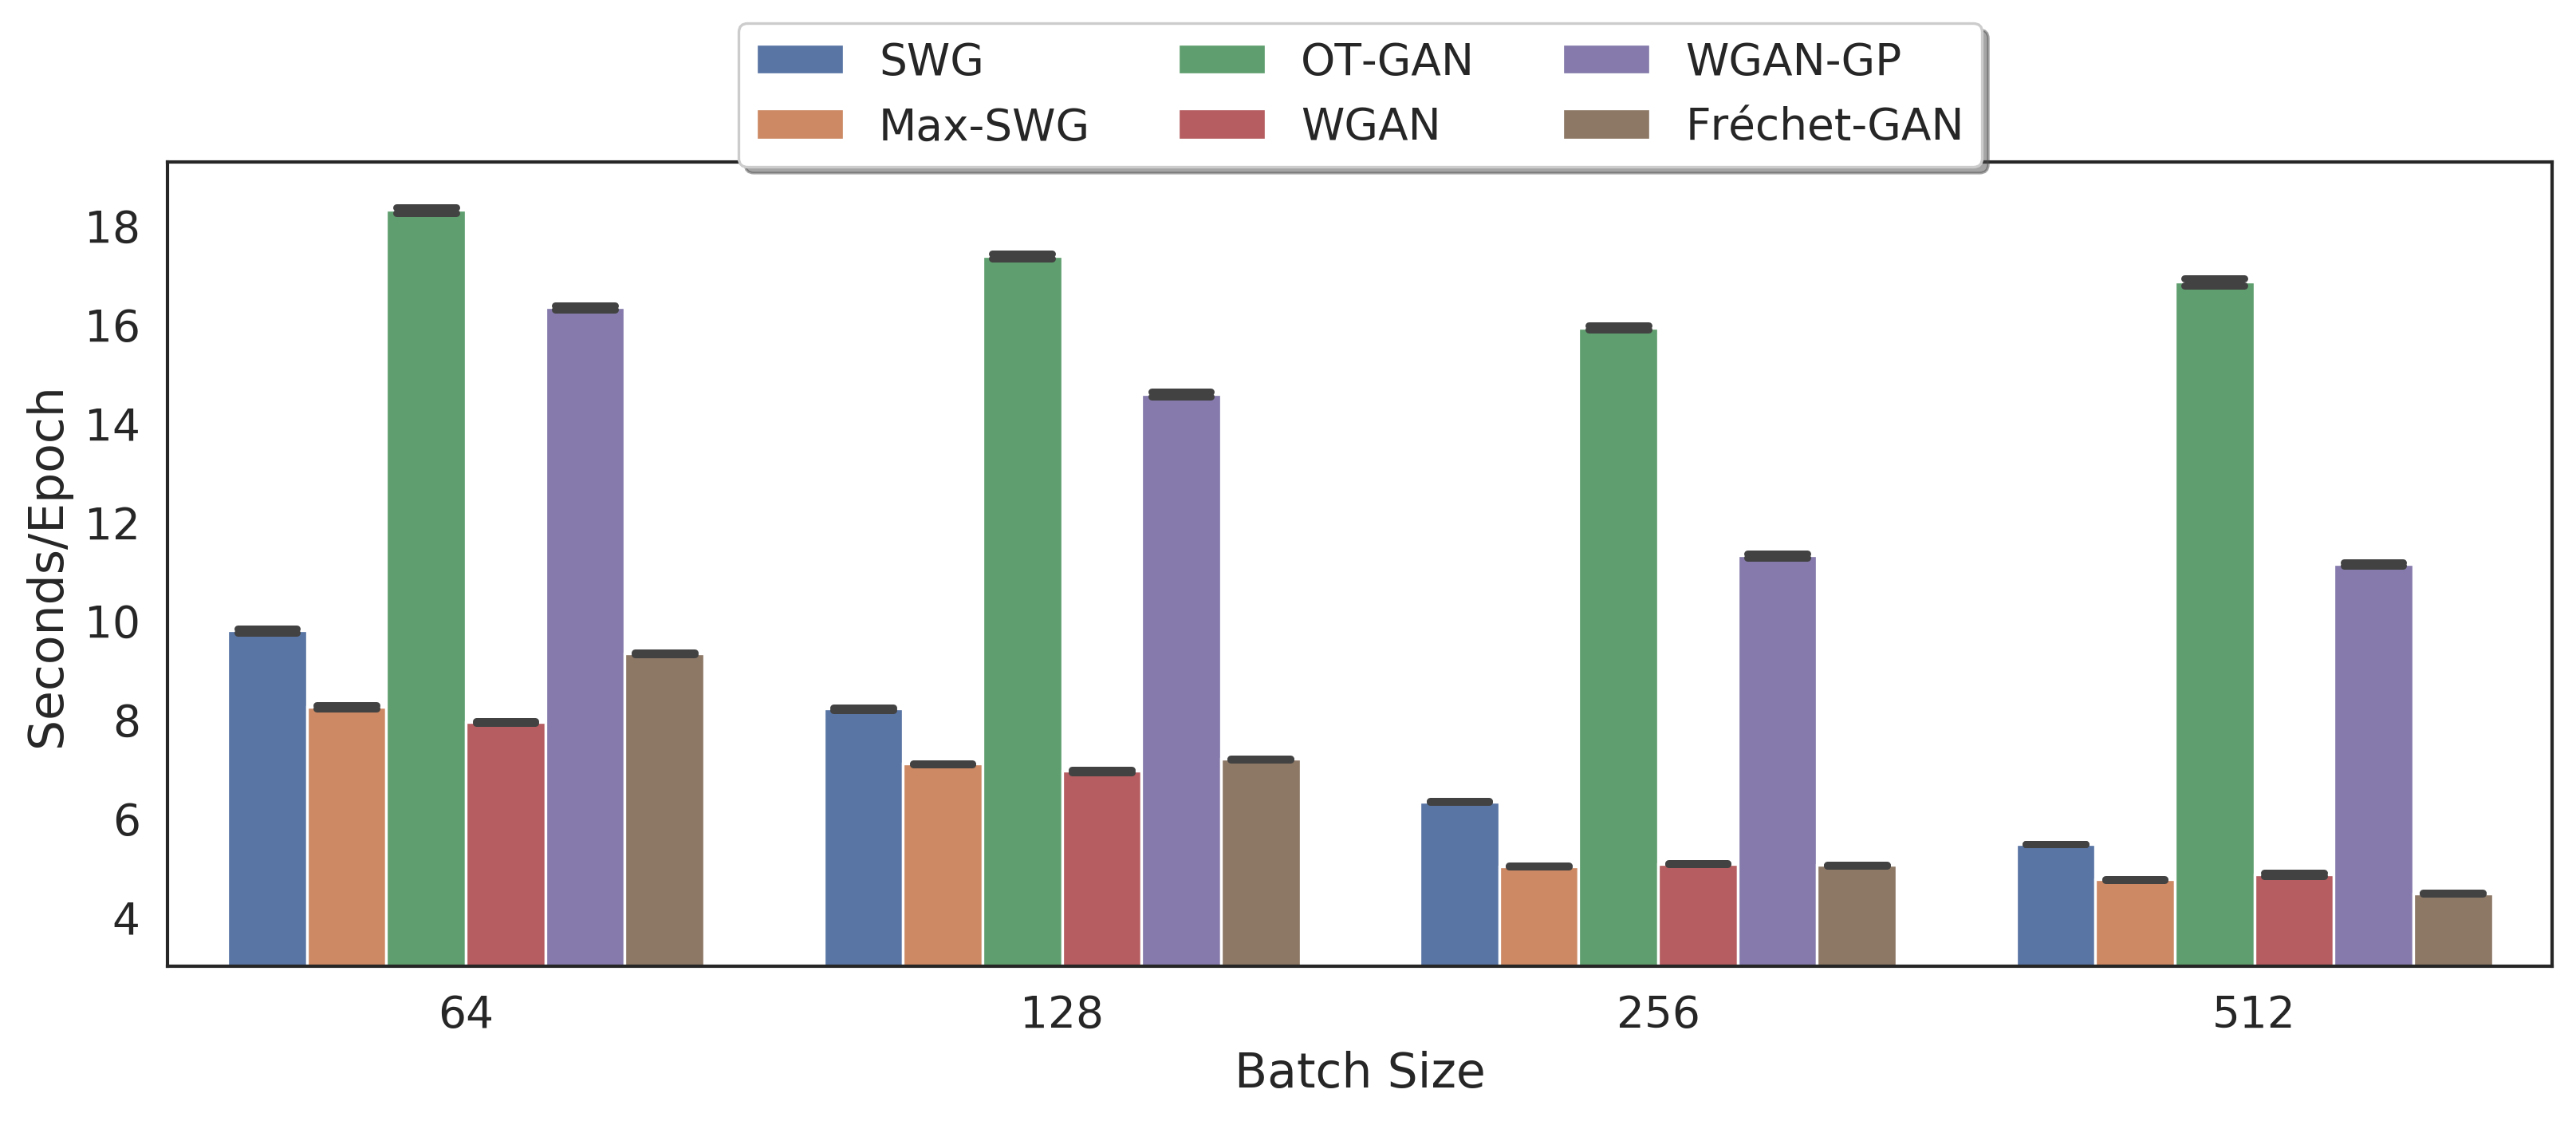}
 }
 \vfill
 
 \subfloat[OT-GAN: Training Time \label{subfig-2:time_lp}]{%
  \includegraphics[width=0.48 \textwidth]{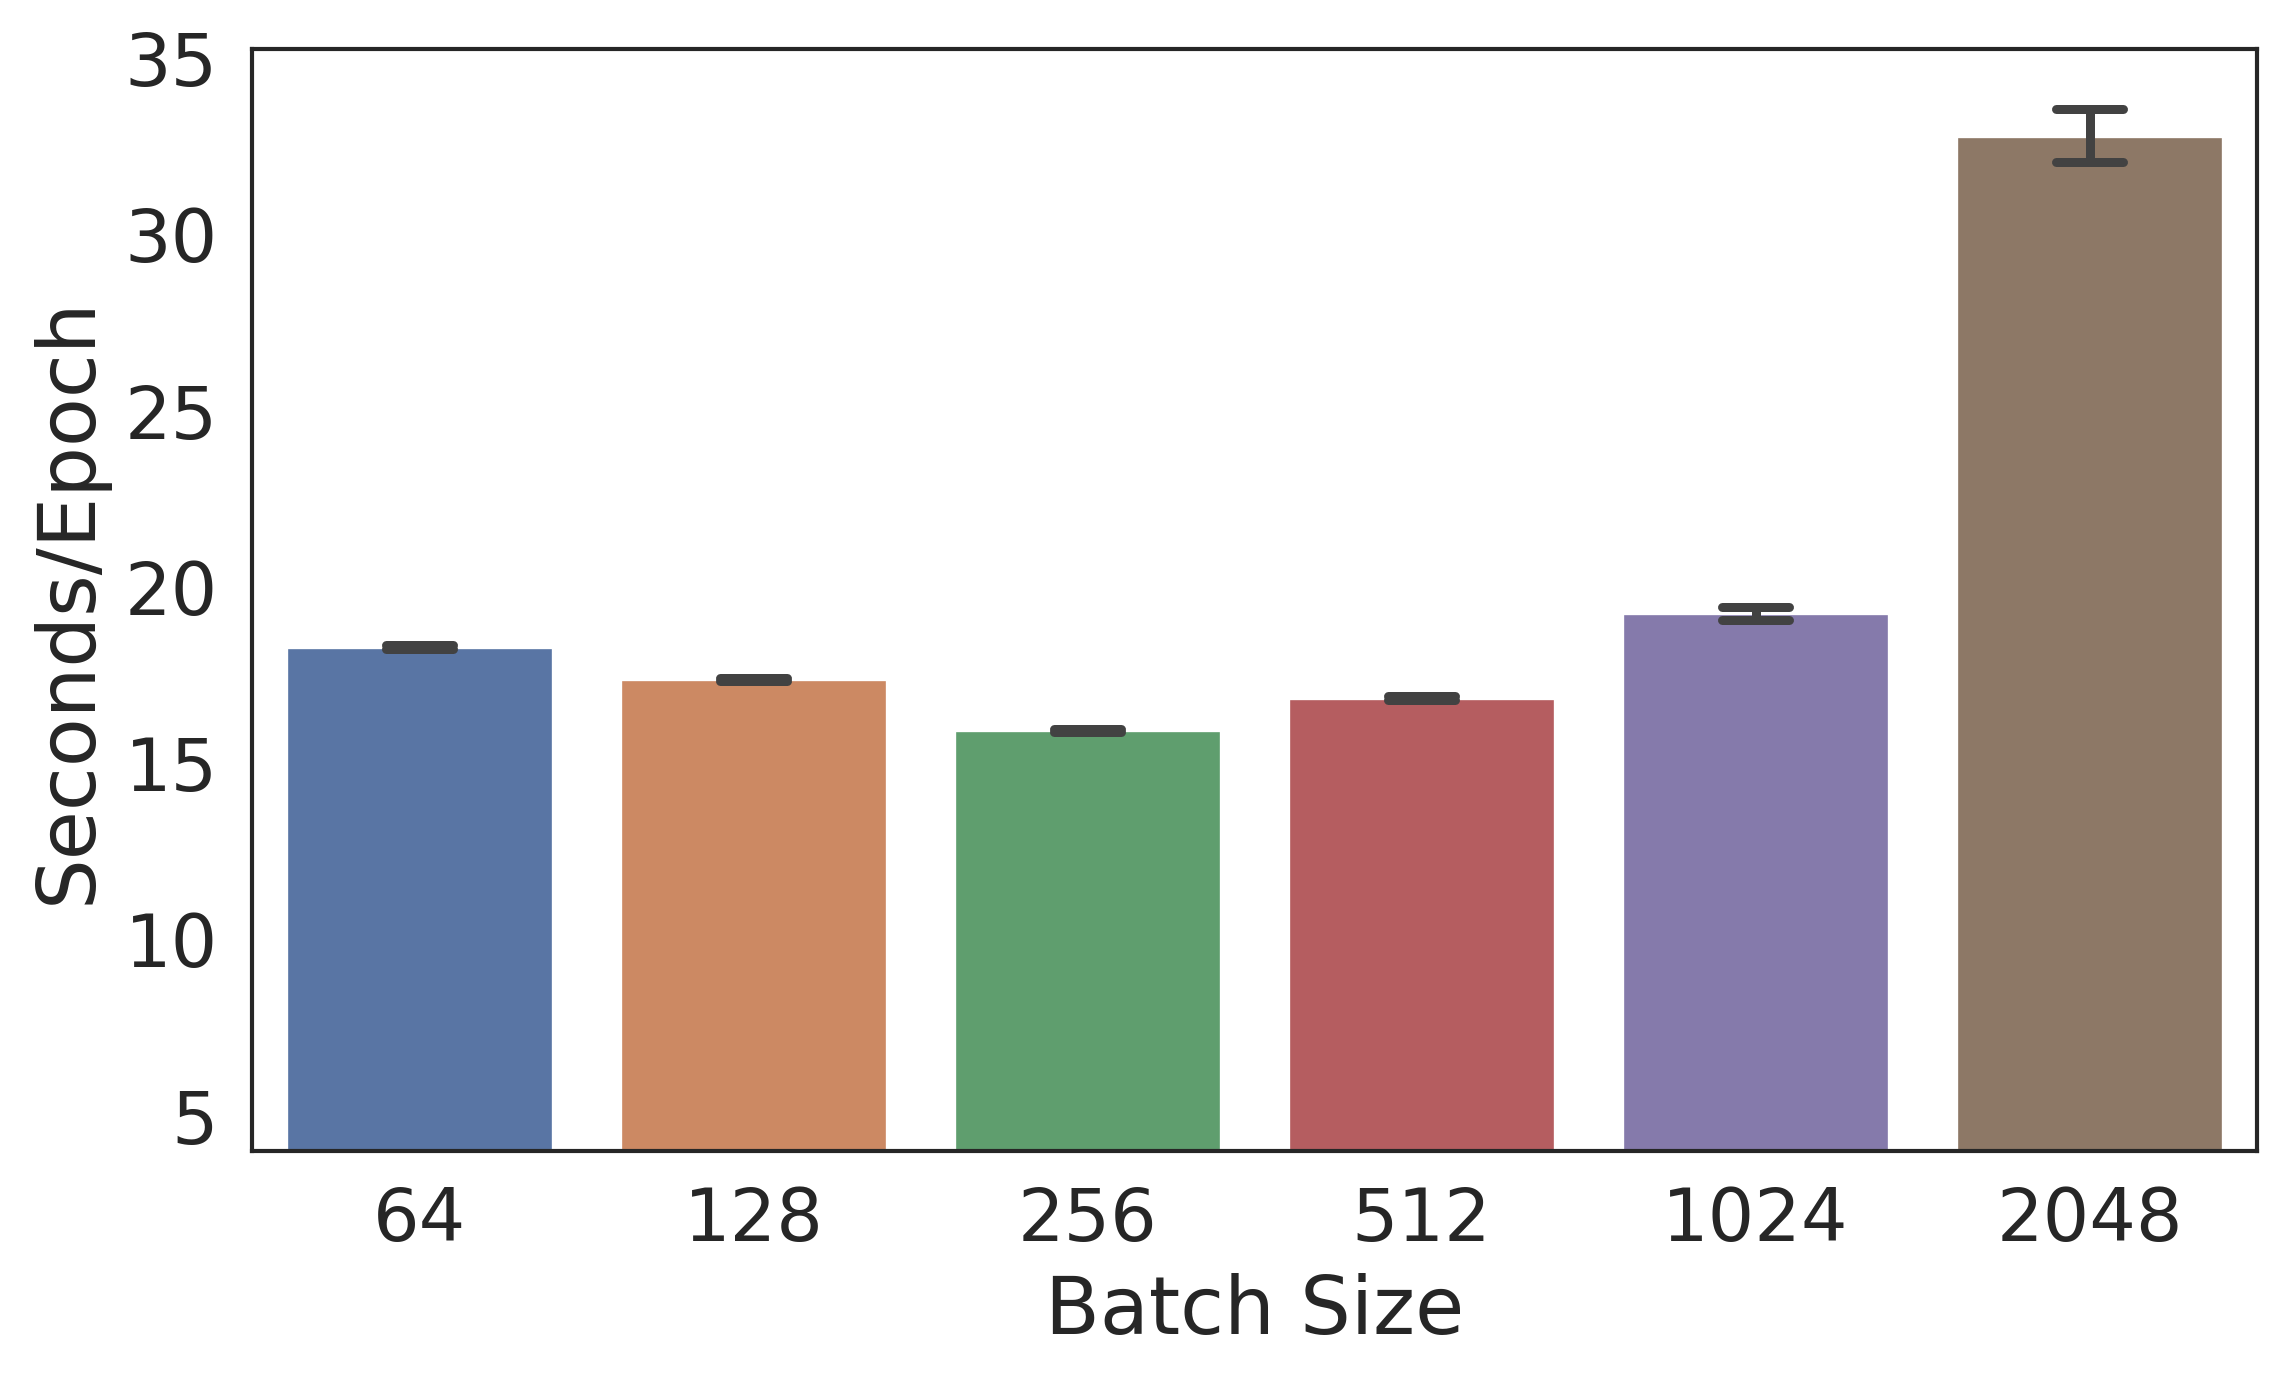}
 }
 \hfill
  
 \subfloat[Fr\'{e}chet-GAN: Training Time \label{subfig-2:time_fgd}]{%
  \includegraphics[width=0.48 \textwidth]{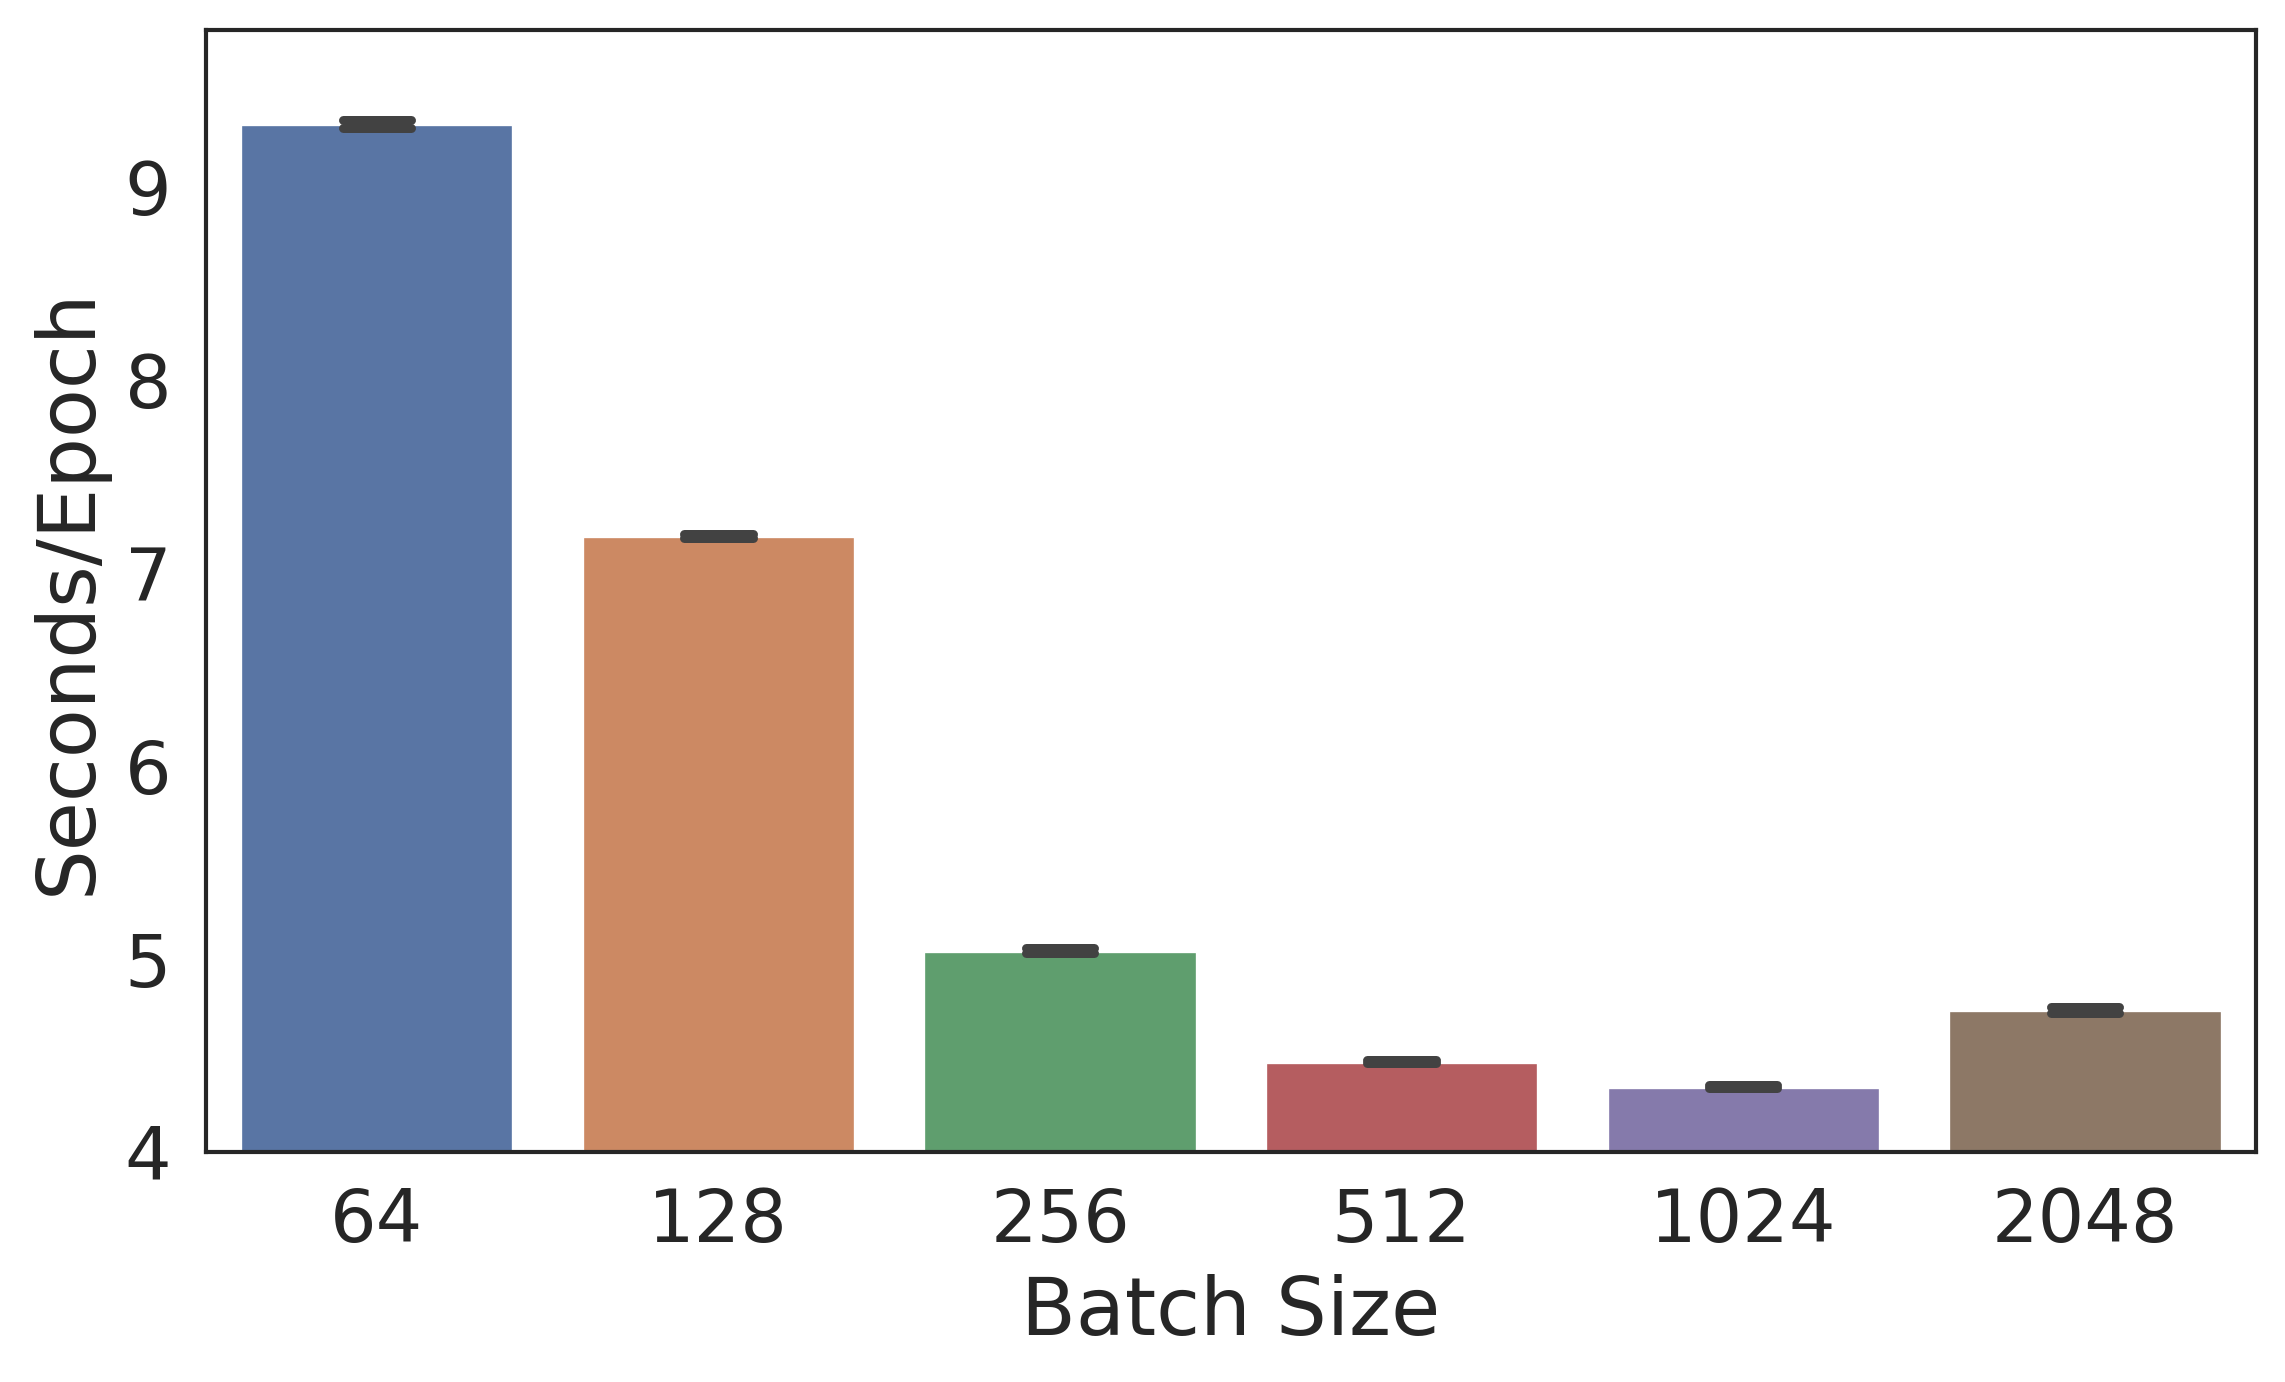}
 }
 \vfill
 
 \subfloat[Fr\'{e}chet-GAN: FID vs. Batch Size \label{subfig-2:fgd_batch_size_fid}]{%
  \includegraphics[width=0.6 \textwidth]{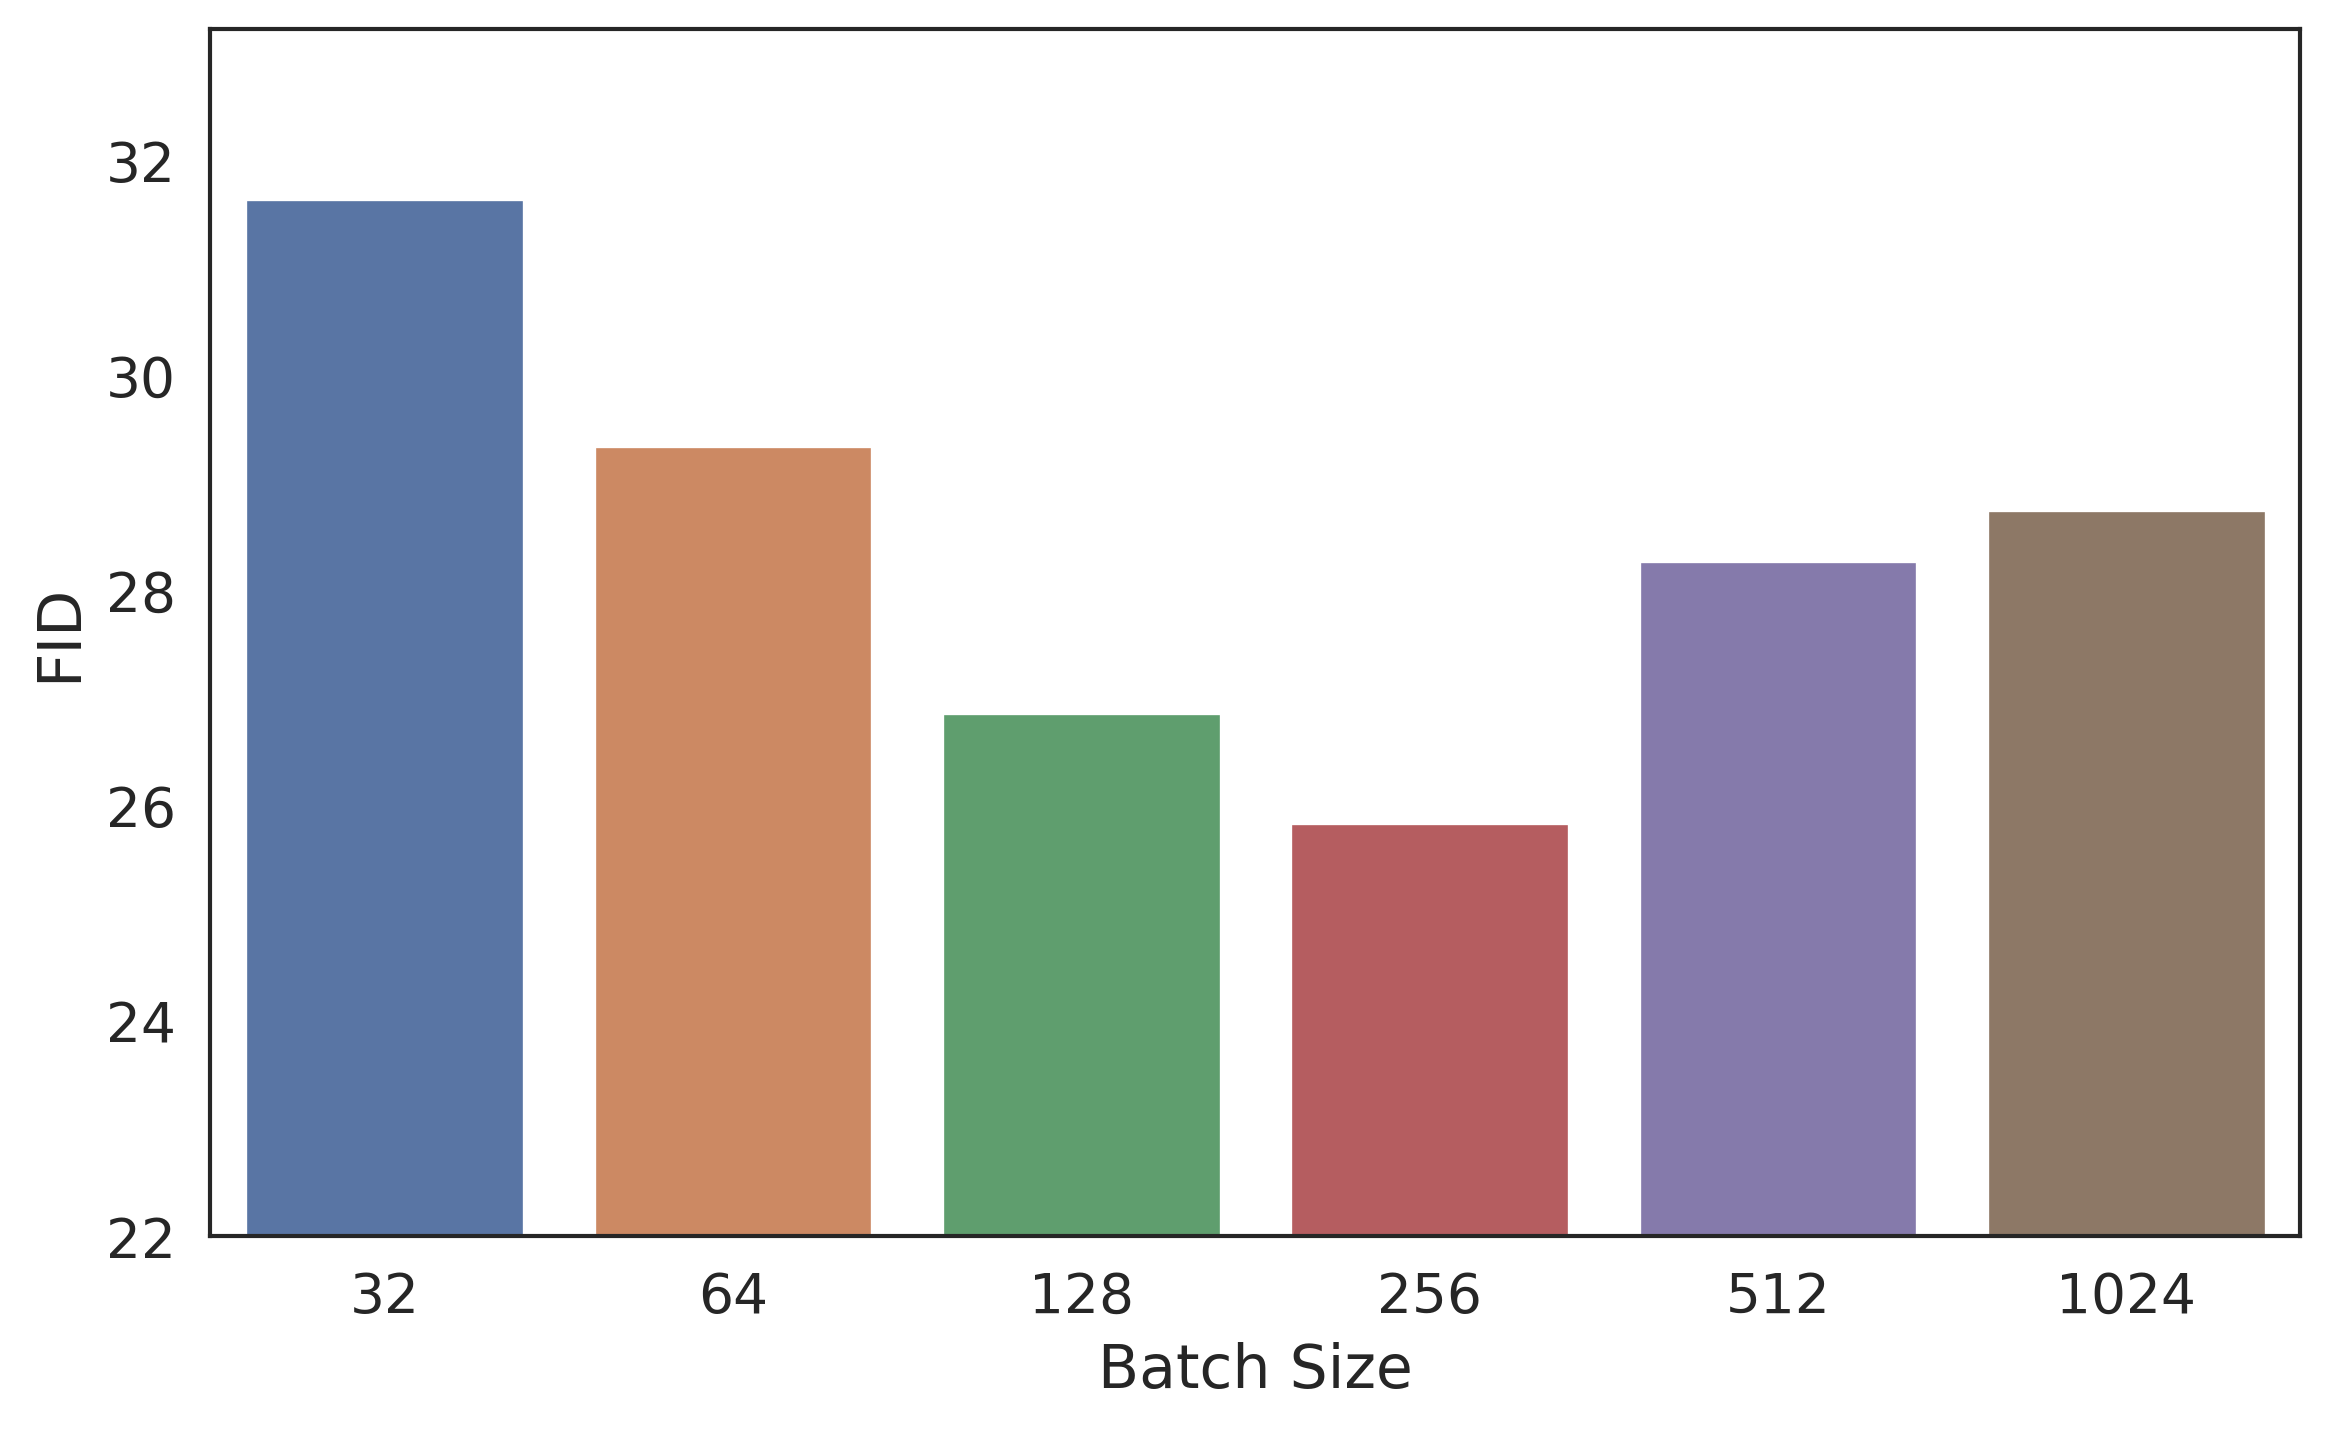}
 }
% \vspace{-5pt}
 \caption{Training time (in seconds) per epoch on the CIFAR-10 dataset.}
 \label{fig:}
\end{figure*}
